# Supplementary material for: A Simple yet Brisk and Efficient Active Learning Platform for Text Classification
Source: arXiv:2102.00426 source file (2021-01-31)
Supplement: Supplementary file 1 [file appendix.tex]

\newpage
\section{Appendix}
\subsection{Active learning experiments and results for insurance data sets}
\subsubsection{Categorizing auto claims loss causes}
Figure \ref{fig:al_san_experiments} (b)-(d) shows the active learning process of binary base classifiers for these three loss causes. In the \textit{Tire Blowout} figure (Figure \ref{fig:al_san_experiments}(b)),  the dynamic lambda curve (purple) arguably has the best AUC below 30\% label, then closely traces the curve of optimal lambda value 0.1 (orange) ; In the \textit{Water Damage} figure (Figure \ref{fig:al_san_experiments}(c)), dynamic lambda AUC curve (purple) becomes second best after 30\%label whereas the optimal lambda value is 1 before 30\%label and 0.1 after; In the \textit{Wind Damage} figure (Figure \ref{fig:al_san_experiments}(d)), dynamic lambda AUC curve (purple) close sly traces the curve of lambda 10 which is the optimal lambda value before 60\% label and becomes the second place after. The curves of different lambda value shows the optimal values of lambda is data set dependent and can also change when the labels accumulated. \textcolor{red}{add explanation that fnol data sets are smaller and consisted of shorter sentences therefore has more variance, as compared to IMDB}. Although dynamic lambda does not always produce the optimal AUC curve, it certainly is a data driven way to approximate the optimal lambda value in the equation \ref{eq:lssvm2}. 
\subsubsection{Property Claims Audit}

\begin{figure*}
{\centering
  \includegraphics[scale=0.32]{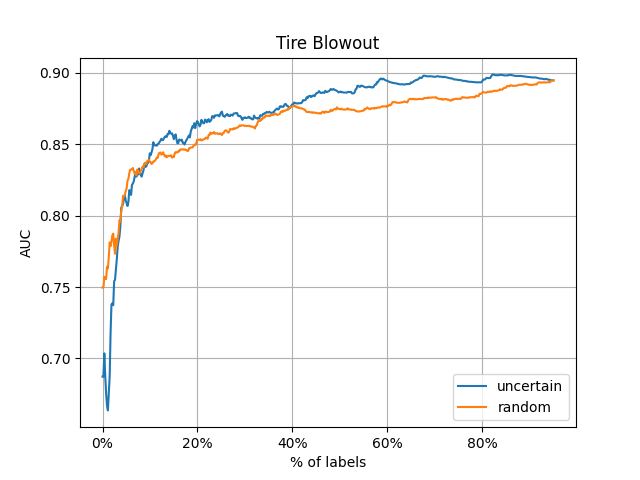} \label{fig:1a}
  \includegraphics[scale=0.32]{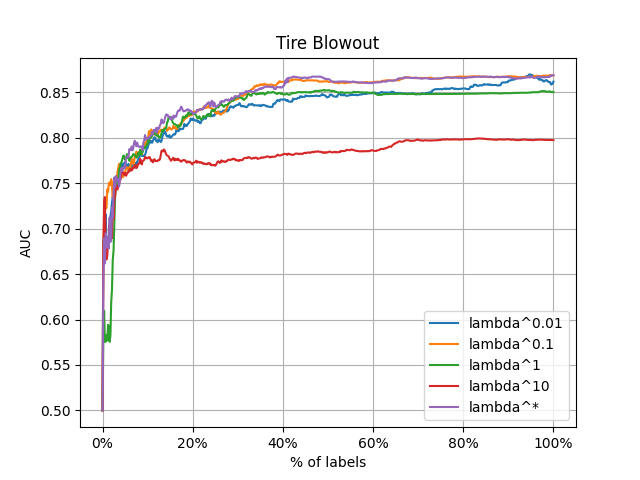}
  \includegraphics[scale=0.32]{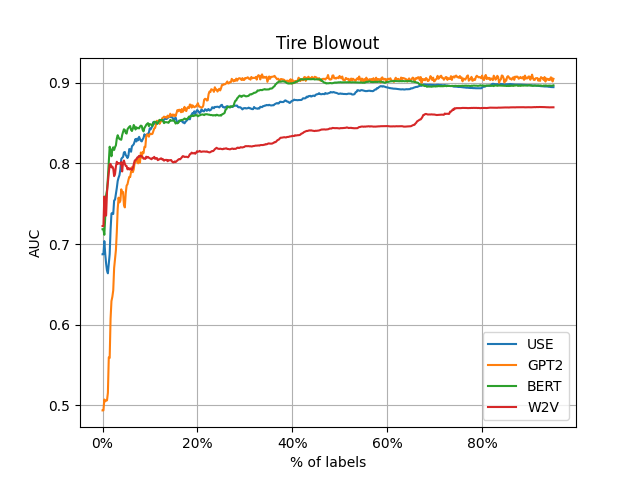}
  \includegraphics[scale=0.32]{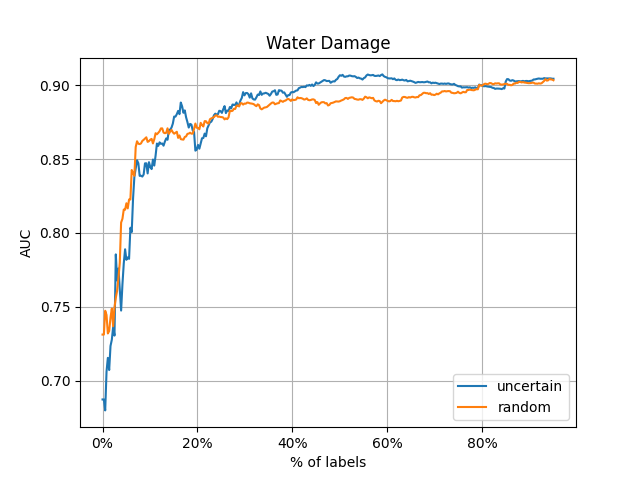}
  \includegraphics[scale=0.32]{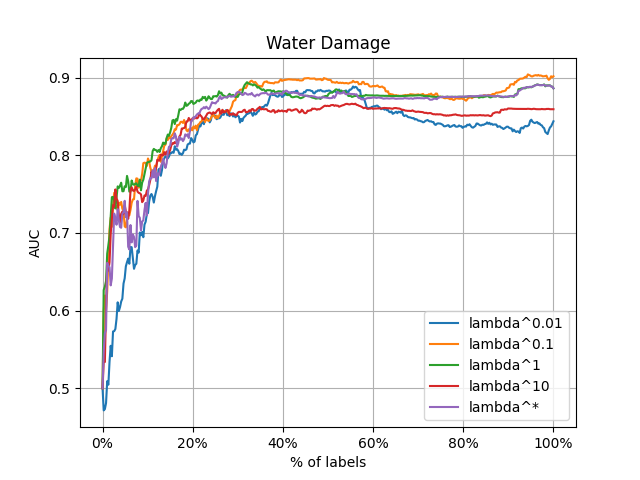}
  \includegraphics[scale=0.32]{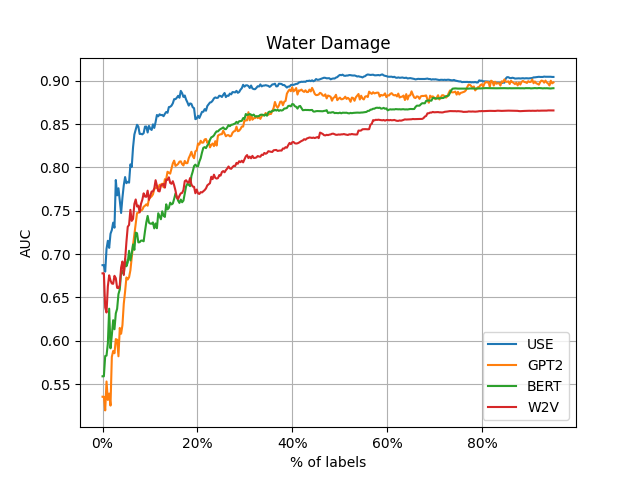}
  \includegraphics[scale=0.32]{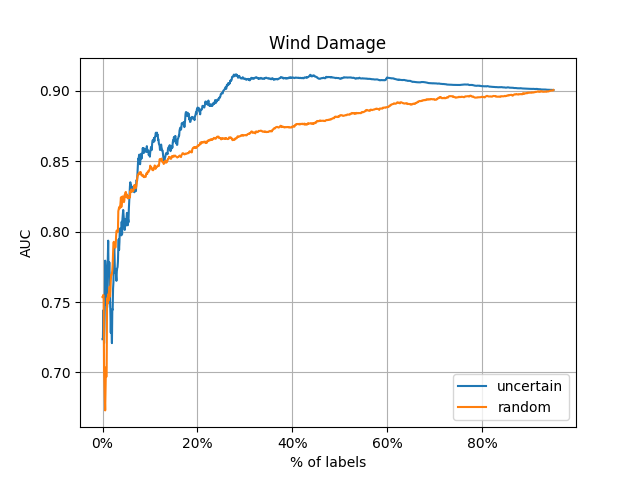} \label{fig:1a}
  \includegraphics[scale=0.32]{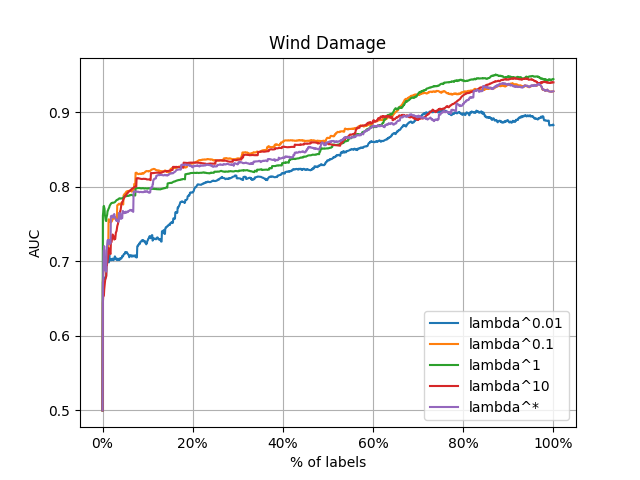}
  \includegraphics[scale=0.32]{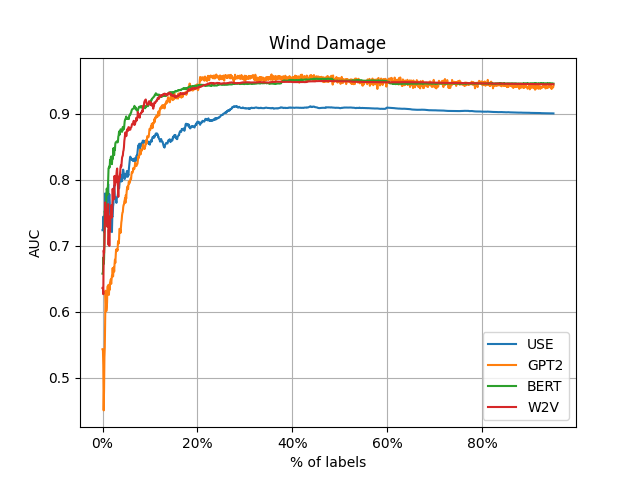}
  \caption{Active learning results for RV claim loss causes: Tire Blowout (a) uncertainty sampling strategy versus random sampling (b) dynamic lambda regularization versus different lambda values (c) language model text representations; Weather Damage (d)-(f); Wind Damage (g)-(i) }
  \label{fig:al_san_experiments}
  }
\end{figure*}

\subsubsection{Model Serving}
A detailed model serving is shown in figure \ref{fig:rocket_deployment}(b).  Executing a Task in Elastic Container Service (ECS).  A cron powered AWS CloudWatch event will run an AWS Lambda function on pre-defined schedule. AWS Lambda prepares a batch document and uploads that batch document to S3. This Bucket has object logging enabled that means all actions on S3 Objects are recorded in AWS CloudTrail as Amazon S3 Data Events. The CloudTrail event selector is configured to select the S3 Bucket/prefixes that are associated with batch document upload. These AWS CloudTrail events are sent to CloudWatch Logs that can trigger an alarms in predefined CloudWatch event rule. The target of CloudWatch event rule is a scheduling an ECS task in ECS cluster powered by Fargate. ECS task pulls the container from ECR (Elastic Container Registry) and executes the task with supplied event data which has the name and location of the batch document that executed this task.  

The ECS task will then read files uploaded in S3 and process documents using FICO. Those weights of models in FICO are small enough to be packaged into the same docker image. This task typically took less than 4GB RAM and 2VCPUs, so one ECS task can appropriately handle the run time requirements. After the FICO process, the time for inference or scoring a document takes seconds since we used a linear model. This design will meet the requirements of 48 hours SLA if processing a batch of thousands of short documents. The scoring results, with the meta data and content of the documents are stored in AWS Managed Relational Database Service (RDS). In case of errors, the ECS would send an an error handled response to an external IT service management tool called ServiceNow via AWS Simple Notification Service (SNS). This response can be picked up by engineered on the ServiceNow platform to address any issues with data processing. \par

Saving results in RDS provides the flexibility of slicing and dicing the scoring results in a business friendly metric dashboard using Tableau. Tableau is a data visualization software tool that connects to RDS in real time and displays a summary of information. The model classifies property insurance claims, which have at least one corresponding comments. Using this software, two dashboards were developed to show the model's classification results at a claim and comment level by filtering by the batch date, confidence threshold, and topic. Figure ? categorizes Relevant Claims as the items the model scored above the selected confidence threshold. This dashboard displays the ratio between non-relevant and relevant claims as well as the magnitude of each category. Figure ? groups comments id with the claim id to display meta information including comment date, peril, insured name, date of loss, and the topic score (model prediction). Business users would be able easily view at a detailed and summary level of property insurance data. Users are also able to export information from each Tableau dashboards for their own records.
